# Supplementary material for: Topological enslavement in evolutionary games on correlated multiplex networks
Source: arXiv:1705.06972 ancillary file (2018-04-23)
Supplement: Supplementary file 1 [file SI.pdf]

# Supplementary Materials for "Topological enslavement in evolutionary games on correlated multiplex networks"

Kaj-Kolja Kleineberg[1, *] and Dirk Helbing[1]

[1] *Computational Social Science, ETH Zurich, Clausiusstrasse 50, CH-8092 Zurich, Switzerland*

(Dated: April 23, 2018)

## CONTENTS

I. Generating realistic multiplex networks with geometric correlations 1

II. Public goods game 2

III. Cooperation in a single network 3

IV. Two layer Barabasi-Albert multiplex without correlations 3

V. Additional results 3

VI. Results for $g = 0$ 3

VII. Distribution of cooperation in different layers 4

VIII. Coherence 5

IX. Robustness of results 8
- A. Results for imitate the best 8
- B. No layer normalization 8

References 8

## I. GENERATING REALISTIC MULTIPLEX NETWORKS WITH GEOMETRIC CORRELATIONS

The geometric multiplex model is based on the (single-layer) network construction procedure of the newtonian $\mathbb{S}^1$ [1] and hyperbolic $\mathbb{H}^2$ [2] models. The two models are isomorphic and here we present the results for the $\mathbb{H}^2$ version. The construction of a network of size $N$ proceed first by assigning to each node $i = 1, \dots, N$ its popularity and similarity coordinates $r_i, \theta_i$ and subsequently, connecting each pair of nodes $i, j$ with probability $p(x_{ij})$ given by the Fermi-Dirac distribution

$$p(x_{ij}) = 1/(1 + e^{\frac{1}{2T}(x_{ij}-R)}) \,, \tag{1}$$

where

$$x_{ij} = \cosh^{-1}\left(\cosh r_i \cosh r_j - \sinh r_i \sinh r_j \cos \Delta\theta_{ij}\right) \tag{2}$$

is the hyperbolic distance between the nodes and $R \propto \ln N$ [2]. $\Delta\theta_{ij} = |\pi - |\pi - |\theta_j - \theta_i|||$ denotes the angular distance between nodes $i$ and $j$. The temperature parameter $\bar{T}$ controls the level of clustering in the network [3]. The average clustering $\bar{c}$ is maximized at $T = 0$, linearly decreases to zero with $\bar{T} \in [0, 1)$, and is asymptotically zero if $\bar{T} > 1$. As $\bar{T} \to 0$ the connection probability becomes the step function $p(x_{ij}) \to 1$ if $x_{ij} \leq R$, and $p(x_{ij}) \to 0$ if $x_{ij} > R$. It has been shown that the $\mathbb{S}^1$ and $\mathbb{H}^2$ models can build synthetic networks reproducing a wide range of structural characteristics of real networks, including power law degree distributions and strong clustering [1, 2]. The use of these models for the single-layer networks allows for radial and angular coordinate correlations across the different layers.

---

* kkleineberg@ethz.ch

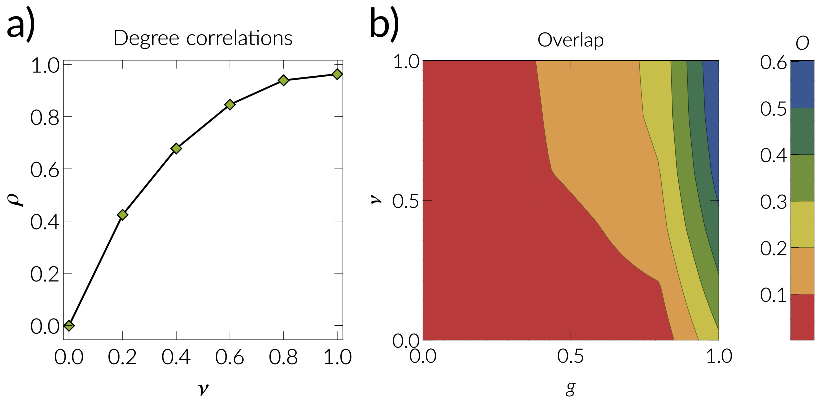


Figure 1. Results for synthetic two-layer multiplexes generated with the model described in the text averaged over 100 realizations of the multiplex construction procedure. Layers have $N = 4000$ nodes, power-law exponents $\gamma = 2.6$, and mean local clustering coefficient 0.4. **(a)** shows degree correlations $\rho$ (Pearson correlation coefficient between the degrees of nodes in layer 1 and 2) as a function of the parameter $\nu$. **(b)** shows the overlap $O$, defined as the fraction of the number of common edges in both layers divided by the maximum of the number of edges in layer 1 and 2, as a function of the parameters $g$ and $\nu$.

The level of these correlations can be controlled by model parameters $\nu \in [0, 1]$ and $g \in [0, 1]$, without affecting the topological structure of the single layers. The radial correlations, related to the node's degree, increase with parameter $\nu$ (see Fig. 1a). At $\nu = 0$ there are no radial correlations, while at $\nu = 1$ radial correlations are maximized. Similarly, the angular correlations increase with parameter $g$. At $g = 0$ there are no angular correlations, while at $g = 1$ angular correlations are maximized. See [4] for details.

In Fig. 1 we show the resulting degree correlations and overlap in the multiplex as a function of the mentioned parameters $\nu$ and $g$.

## II. PUBLIC GOODS GAME

In the version of the public goods game considered here [5], individuals play in different overlapping groups. A node with degree $k_i$ plays in $G = k_i + 1$ groups, centered around each of its neighbors and the node $i$ itself. A group centered around node $i$ consists of the node itself and its $k$ neighbors, hence it has size $k_i + 1$. Each node can cooperate ($s_i = 1$) or defect ($s_i = 0$) in each layer independently. Cooperators contribute to public pools collected in the groups with a total amount $c$, which we set to 1. Cooperators distribute their contribution equally among the $G$ groups they participate in, thus they invest $c/(k_i + 1)$. We denote the common pool in the group centered around node $i$ in layer $l$ as $\mathcal{G}_{i,l}$. The whole amount in this pool is then

$$\mathcal{G}_{i,l} = \frac{c}{k_{i,l} + 1} s_{i,l} + \sum_{j \in \mathrm{NB}(i,l)} \frac{c}{k_{j,l} + 1} s_{j,l} \,, \tag{3}$$

where $k_{i,l}$ denotes the degree of node $i$ in layer $l$ and $\mathrm{NB}(i, l)$ is the set of neighbors of node $i$ in layer $l$. The total amount in the pool is multiplied by $r$ and distributed equally among all nodes in the group. Hence, node $j$ obtains the payoff

$$\hat{\pi}_{i,j,l} = \frac{r\mathcal{G}_{i,l}}{k_i + 1} - \frac{c}{k_j + 1} s_{j,l} \tag{4}$$

from the group centered around $i$ in layer $l$. Summing up the payoffs in each group and each layer then yields the total payoff of node $i$

$$\Pi_i = \sum_{l=1}^{n_l} \left[ \hat{\pi}_{i,i,l} + \sum_{j \in \mathrm{NB}(i,l)} \hat{\pi}_{j,i,l} \right] . \tag{5}$$

After one round of the game, which consists of playing one public goods game in each of the groups, we perform an update step in the same way as explained in the main manuscript. After each round nodes update their strategy, we reset the payoffs and proceed with the next round.

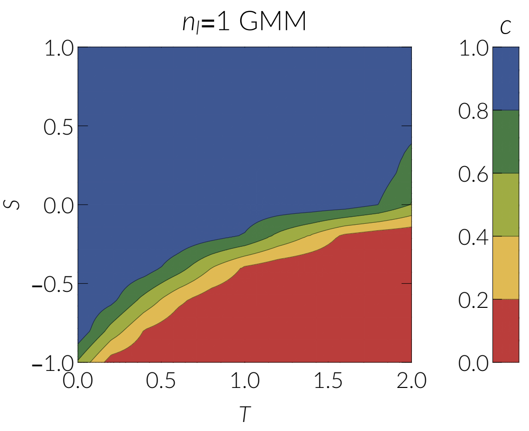


Figure 2. Final average cooperation as a function of the payoff parameters $T$ and $S$ in a single layer. The network has $N = 4000$ nodes, power-law exponent $\gamma = 2.6$, and mean local clustering coefficient 0.4.

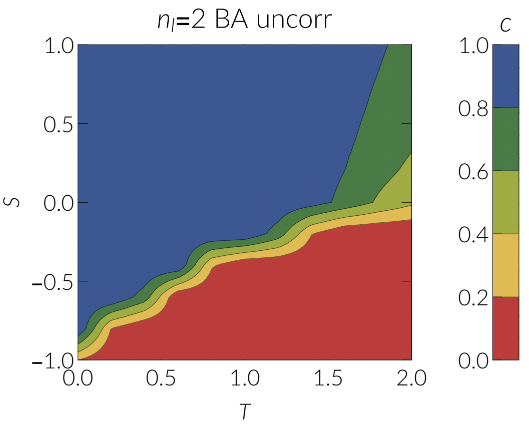


Figure 3. Final average cooperation as a function of the payoff parameters $T$ and $S$ in an uncorrelated two layer multiplex that consists of two Barabasi-Albert network layers. Each layer has $N = 4000$ nodes.

## III. COOPERATION IN A SINGLE NETWORK

Fig. 2 shows the final average cooperation in a single network generated with the model described in the main manuscript, and for the same parameters regarding the single layers as in Fig. 4 in the main manuscript.

## IV. TWO LAYER BARABASI-ALBERT MULTIPLEX WITHOUT CORRELATIONS

Fig. 3 shows results for a two layer Barabasi-Albert multipex without degree correlations.

## V. ADDITIONAL RESULTS

Fig. 4 shows results for additional parameters combinations using the geometric multiplex model.

## VI. RESULTS FOR $g = 0$

Figs. 5 and 6 show results for $g = 0$ similar to Figs. 5 and 6 in the main manuscript.

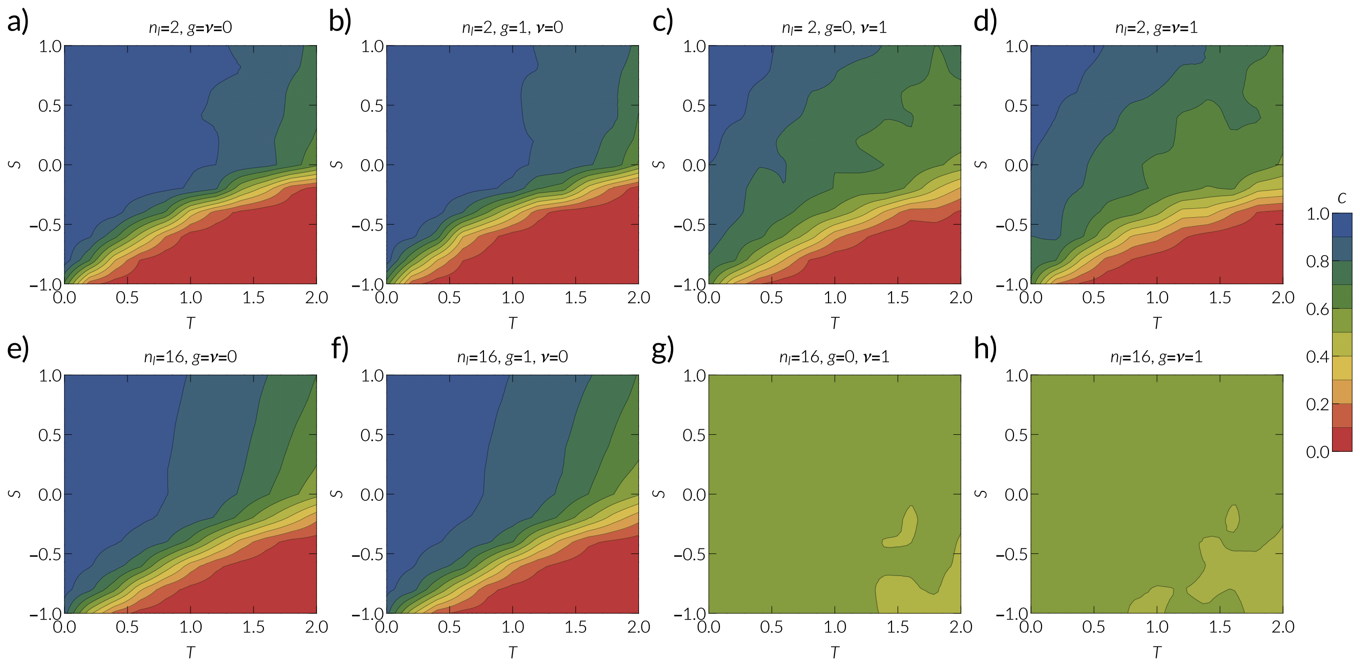


Figure 4. Mean final cooperation (color coded) as a function of the game payoff parameters $T$ and $S$. Results are averaged over 100 realizations. Networks are generated with the model described in the text. Layers have $N = 4000$ nodes, power-law exponents $\gamma = 2.6$, and mean local clustering coefficient 0.4. **(a-d)** are for $n_l = 2$ layers, and **(e-h)** are for $n_l = 16$ layers. **(a)** and **(e)** show no correlations ($g = \nu = 0$, **(b)** and **(f)** show only similarity correlations ($g = 1$), **(c)** and **(g)** show only degree correlations ($\nu = 1$), **(d)** and **(h)** show degree and similarity correlations ($g = \nu = 1$).

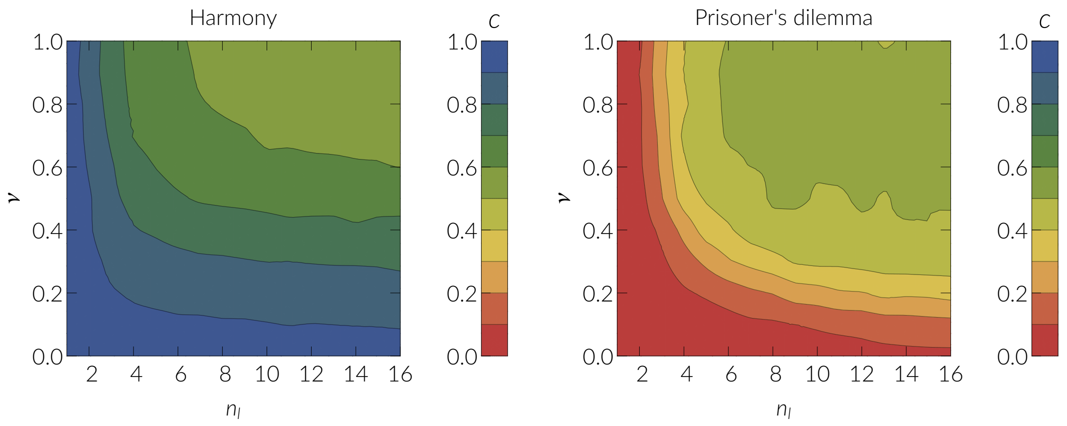


Figure 5. The same as in Fig. 5 of the main manuscript but for $g = 0$.

## VII. DISTRIBUTION OF COOPERATION IN DIFFERENT LAYERS

In Fig. 7 we show the distribution of average cooperation in different layers for the harmony game. From left to right we increase the strength of the degree correlations. We observe that for low values of $\nu$ layers are close to fully cooperative, and as $\nu$ is increased one eventually observes that layers are mainly cooperative with probability $c_0$ and mainly defective with probability $1 - c_0$.

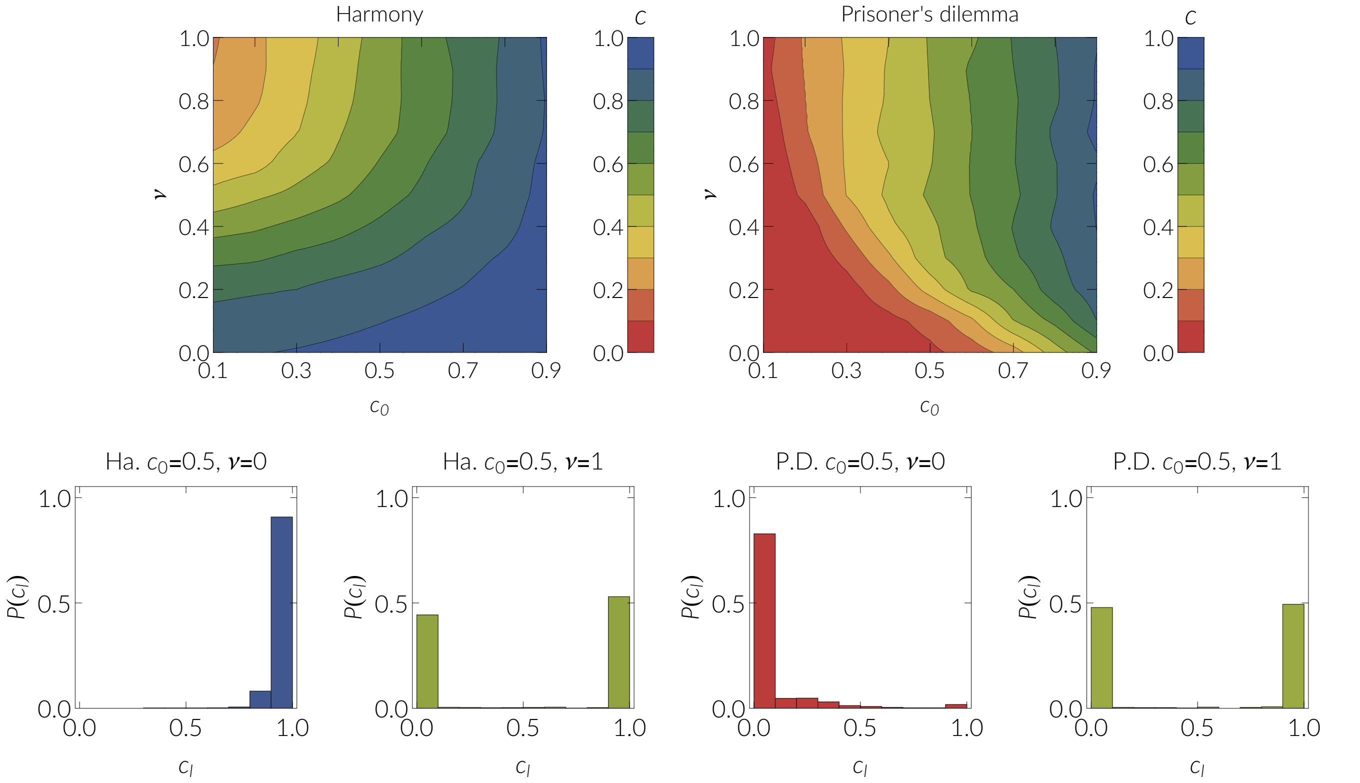


Figure 6. The same as in Fig. 6 of the main manuscript but for $g = 0$.

## VIII. COHERENCE

Let us quantify the strategic coherence of individuals in different layers. Therefore, we define the mean coherence defined as [6]

$$\xi = \frac{1}{n}\sum_{i=1}^{n}\xi_i\,, \quad \xi_i = \left|\frac{1}{n_l}\sum_{j=1}^{n_l} s_i^{(l)}\right|\,, \tag{6}$$

where $n$ is the number of nodes, $n_l$ the number of layers, and $s_i^{(l)}$ the state of the node $i$ in layer $l$, such that

$$s_i^{(l)} = \begin{cases} 1 & \text{for cooperate} \\ -1 & \text{for defect} \end{cases} \,. \tag{7}$$

This definition ensures that if each node has the same state in all the layers we have full coherence, $\xi = 1$, and if node states are alternating, then we have $\xi = 0$.

In Fig. 9 we show results of the coherence. We observe that in the parameter region where topological enslavement occurs, i.e. for large $\nu$ and $n_l$, we observe a low coherence. This is in agreement with the observation that whereas the mean cooperation in the system is $c \approx c_0$, each layer is either nearly fully cooperative or defective. The probability that a layer is cooperative is then approximately $c_0$.

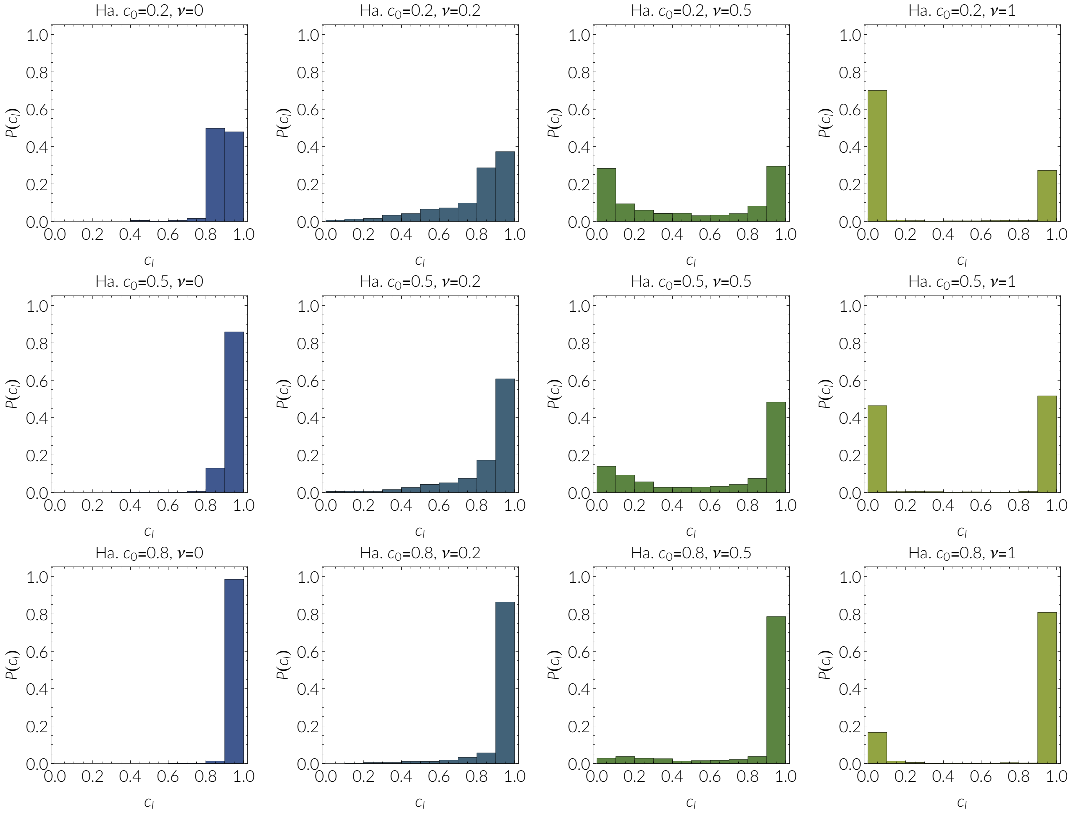


Figure 7. Distribution of average cooperation in individual layers for different initial conditions and strengths of degree correlations for the harmony game and 16 layers over 60 realizations.

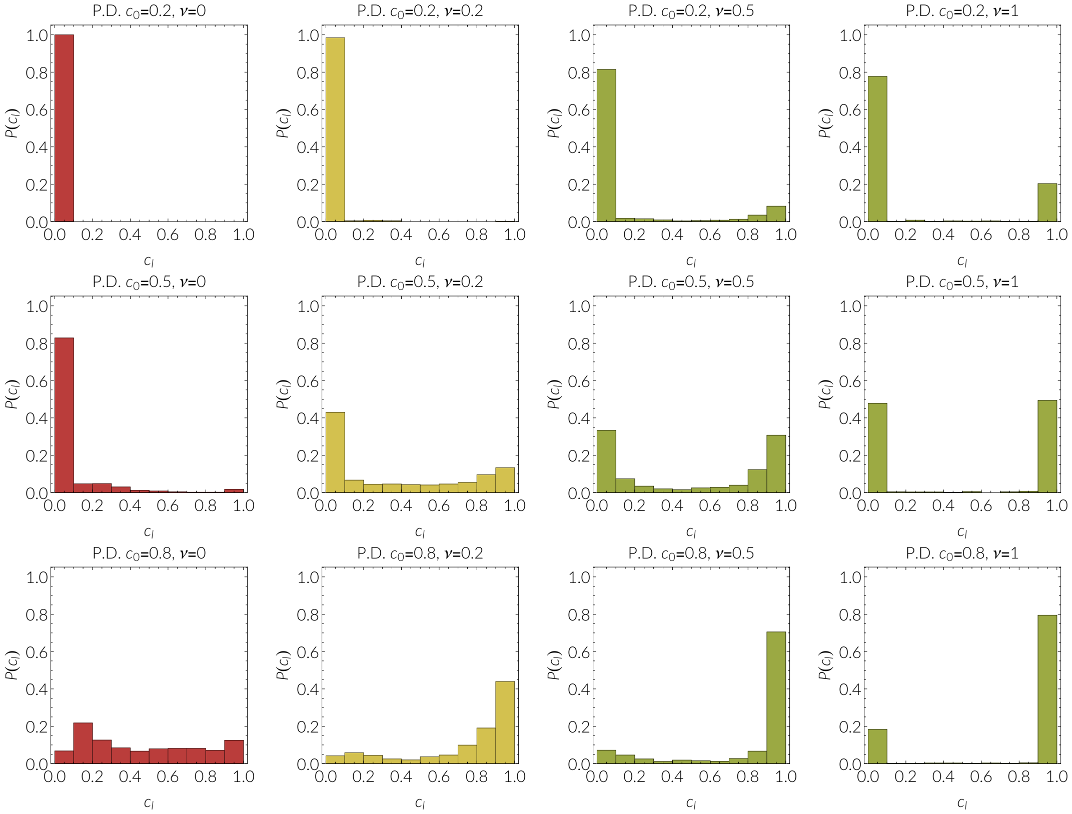


Figure 8. Distribution of average cooperation in individual layers for different initial conditions and strengths of degree correlations for the prisoner's dilemma game.

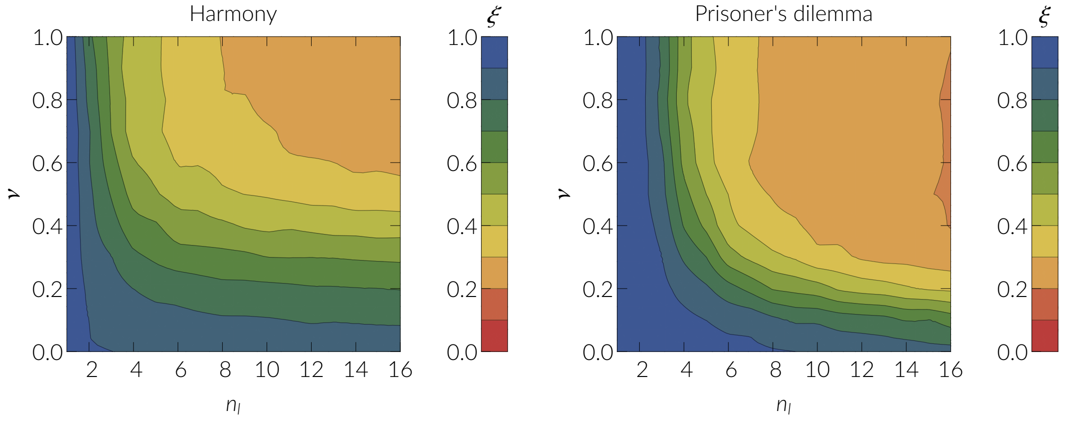


Figure 9. Coherence $\xi$ from Eq. (6) for the harmony and prisoner's dilemma game as in the main manuscript as a function of the number of layers.

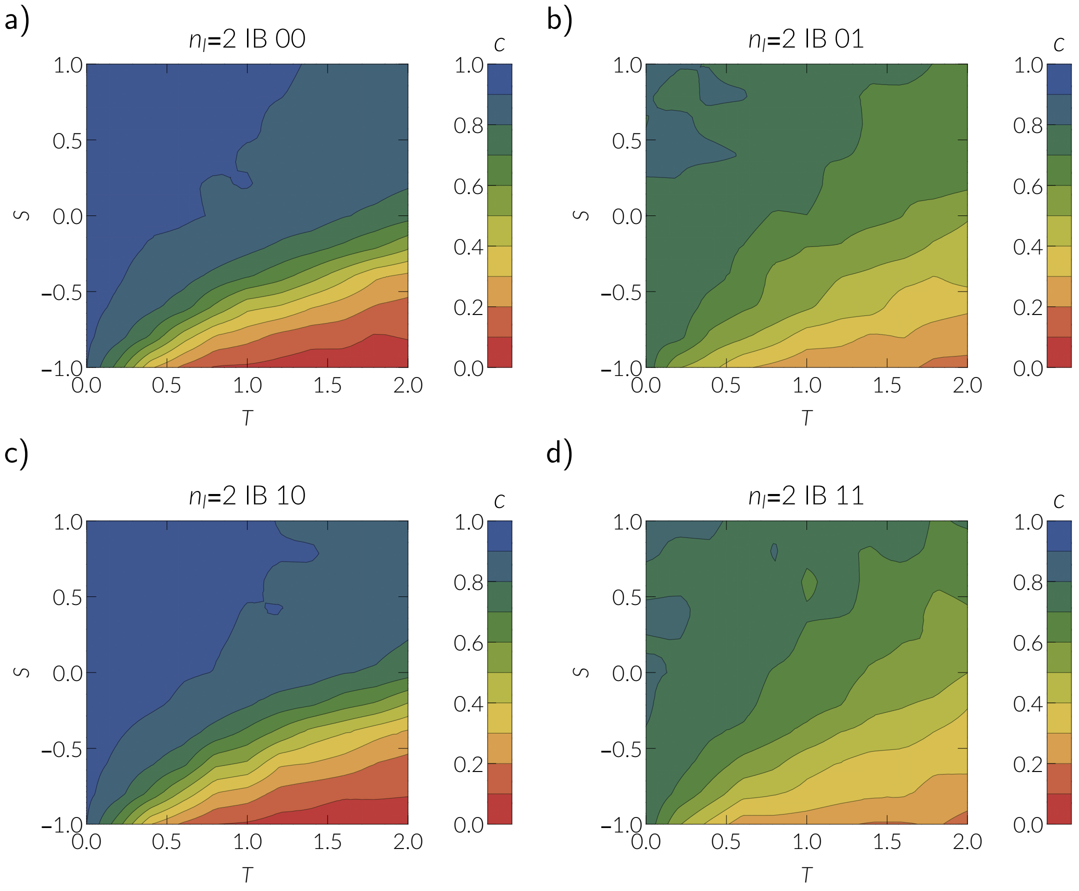


Figure 10. The same as in Fig. 1 of the main manuscript, but only for two layers. **a)** $g = \nu = 0$. **b)** $g = 0, \nu = 1$. **c)** $g = 1, \nu = 0$. **d)** $g = \nu = 1$.

## IX. ROBUSTNESS OF RESULTS

### A. Results for imitate the best

Here, we investigate different update rules. In particular, we consider "imitate the best" (IB) dynamics, where instead of selecting a random neighbor each node imitate the strategy of her neighbor with the highest payoff in the chosen layer. If the focal individual herself has a higher payoff than the most successful neighbor, she keeps her strategy.

We find a qualitatively similar behavior as for the Fermi rule used in the main manuscript (see Fig. 10 and 11)

### B. No layer normalization

In the main manuscript, we have normalized the overall payoff by the number of layers, $\Pi_i = \frac{1}{n_l}\sum_{l=1}^{n_l} \pi_{i,l}$. Here, we show that the normalization by the number of layers does not alter the results. In particular, we replace the previous expression with $\Pi_i = \sum_{l=1}^{n_l} \pi_{i,l}$. Indeed, Fig. 12 shows that the observed behavior is similar to the one from the main manuscript.

[1] M. Ángeles Serrano, Dmitri Krioukov, and Marián Boguñá, "Self-Similarity of Complex Networks and Hidden Metric Spaces," Phys. Rev. Lett. **100**, 078701 (2008).
[2] Dmitri Krioukov, Fragkiskos Papadopoulos, Maksim Kitsak, Amin Vahdat, and Marián Boguñá, "Hyperbolic geometry of complex networks," Phys. Rev. E **82**, 036106 (2010).

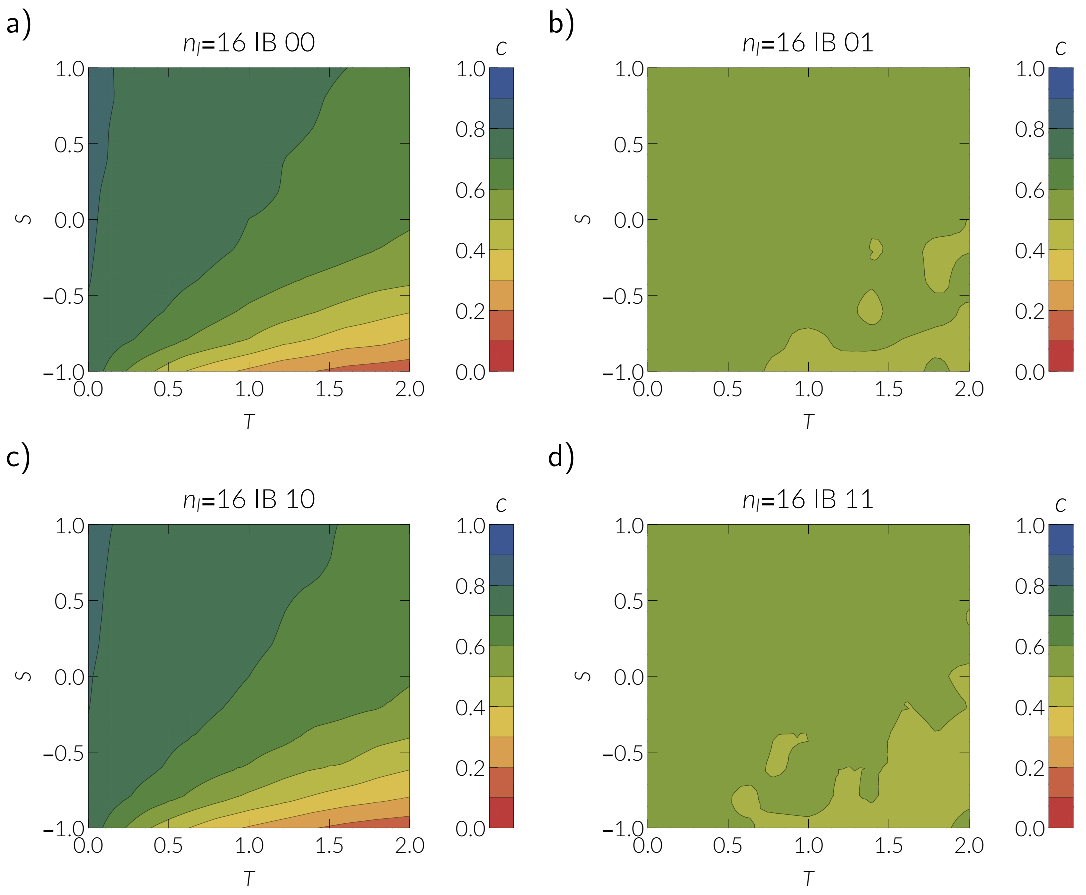


Figure 11. The same as in Fig. 1 of the main manuscript, but only for 16 layers. **a)** $g = \nu = 0$. **b)** $g = 0, \nu = 1$. **c)** $g = 1, \nu = 0$. **d)** $g = \nu = 1$.

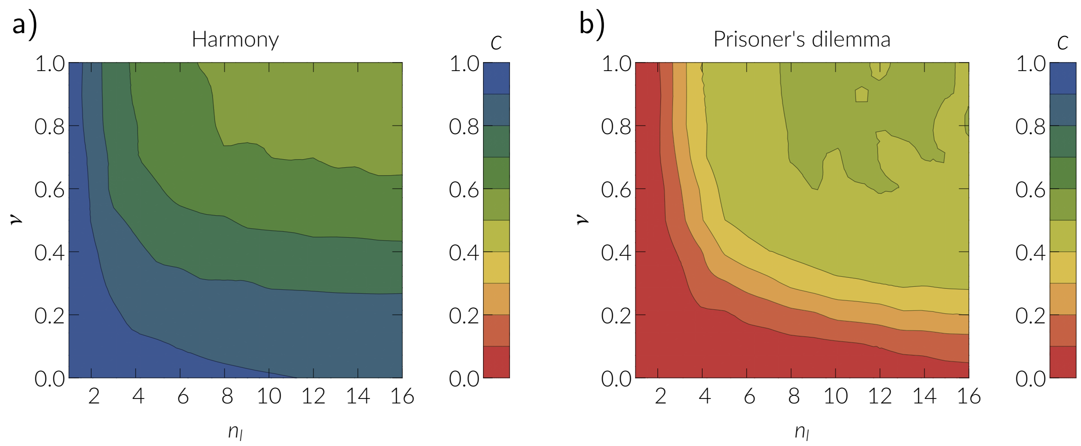


Figure 12. The same as Fig. 4 in the main manuscript, but without normalizing payoffs by the number of layers (see text). **a)** Shows results for the harmony game. **b)** Shows results for the prisoner's dilemma.


[3] S. N. Dorogovtsev, *Lectures on Complex Networks* (Oxford University Press, Oxford, 2010).

[4] Kaj-Kolja Kleineberg, Marián Boguñá, M. Ángeles Serrano, and Fragkiskos Papadopoulos, "Hidden geometric correlations in real multiplex networks," Nat. Phys. **12**, 1076–1081 (2016).

[5] Francisco C Santos, Marta D Santos, and Jorge M Pacheco, "Social diversity promotes the emergence of cooperation in public goods games," Nat. **454**, 213–216 (2008).

[6] Federico Battiston, Matjaž Perc, and Vito Latora, "Determinants of public cooperation in multiplex networks," New Journal of Physics **19**, 073017 (2017).
